# Supplementary material for: JourneyDB: A Benchmark for Generative Image Understanding
Source: arXiv:2307.00716 source file (2023-10-28)
Supplement: Supplementary file 1 [file datasheet.tex]

\section{Datasheet}

\subsection{\centering \centering Motivation}
\subsection*{Why was the dataset created?} 
\noindent While recent advancements in vision-language models have revolutionized multi-modal understanding, it remains unclear whether they possess the capabilities of comprehending the generated images. Compared to real data, synthetic images exhibit a higher degree of diversity in both content and style, for which there are significant difficulties for the models to fully apprehend. To this end, we present a large-scale dataset, JourneyDB, for multi-modal visual understanding in the realm of generative images.
\subsection*{Who created this dataset (\eg which team, research group) and on behalf of which entity (\eg company, institution, organization)?}
\noindent The dataset was created by researchers at the Chinese University of Hong Kong, and was aimed only for scientific research use.

\subsection{\centering Composition}
\subsection*{What do the instances that comprise the dataset represent (\eg
documents, photos, people, countries)? Are there multiple types of instances? (\eg movies, users, ratings; people, interactions between them; nodes, edges)}
\noindent
The instances are prompts and generated images, along with annotations of prompt classification (into content styles), image caption, and visual question answering.

\subsection*{Are relationships between instances made explicit in the data (\eg social network links, user/movie ratings, etc.)?}
\noindent
No. To protect user privacy, we did not include private information in the dataset. But we will provide a service for users to check whether their data is included in this dataset. If they do not hope their images to be included, we will remove them accordingly.

\subsection*{How many instances are there? (of each type, if appropriate)?}
\noindent 
In this version, we collect in total $4,692,751$ images with more than $1024\times1024$ resolution, each with a corresponding text prompt. And there are $1,730,639$ independent prompts. We have $1,472,581$ pieces annotated with GPT-3.5.
% following the procedure described in \Cref{fig:data_collection}. 
Also, there are $5,402$ images filtered by Image-Prompt consistency.
For more details, please refer to the section $3.3$ in the main paper.

\subsection*{What data does each instance consist of? ``Raw'' data (\eg unprocessed text or images) or Features/attributes? Is there a label/target associated with instances? If the instances are related to people, are sub-populations identified (\eg by age, gender, etc.) and what is their distribution?}
\noindent 
Each instance consists of prompts and corresponding images, and the annotations of prompt classification (into content styles), image caption, and visual question answering.

\subsection*{Is any information missing from individual instances? If so, please
provide a description, explaining why this information is missing (\eg
because it was unavailable). This does not include intentionally removed
information, but might include, \eg redacted text.}
\noindent 
Yes. We hide personal information, like user IDs, of the original data to try our best to protect user privacy.

\subsection*{Is everything included or does the data rely on external resources?}
\noindent Yes, the dataset is self-contained.

\subsection*{Are there recommended data splits and evaluation measures? (\eg training, development, testing; accuracy or AUC)}
\noindent 
Yes. We split the dataset into three parts, the training, validation, and testing set. The detailed split parameters are summarized in Table 2 in the main paper. We recommend several evaluation measures for each downstream task in the benchmarks. Please refer to section $4$ for more details. Furthermore, for prompt inversion, we provide a novel metric, namely the Question-Answering Score (QAS), as introduced in \Cref{sec:supp:qas} in this supplementary material.

\subsection*{Are there any errors, sources of noise, or redundancies in the
dataset?}
\noindent Yes. There might be some misalignment between the image and the prompt, which would bring the noise to the annotation.

\subsection*{Is the dataset self-contained, or does it link to or otherwise rely on external resources (\eg websites, tweets, other datasets)?}
\noindent Yes, we have the self-contained data.

\subsection*{Does the dataset contain data that might be considered confidential (\eg data that is protected by legal privilege or by doctorpatient confidentiality, data that includes the content of individuals non-public communications)?}
\noindent 
No, the dataset does not contain confidential data. The collected data are publicly available. 

\subsection*{Does the dataset contain data that, if viewed directly, might be offensive, insulting, threatening, or might otherwise cause anxiety? If so, please describe why.}
\noindent
We have thoroughly revised the dataset to ensure the dataset free from harmful or violent images.

On the one hand, Midjourney itself has provided violence filtering to ensure the presented images and prompts are suitable for the network. On the other hand, we apply an NSFW model on the whole dataset to further analyse the the violence extend of JourneyDB and manually filter the images indeed unsuitable for work.

Images with the NSFW score higher than $0.8$ are likely to be “not-suitable-for-work” images, while the NSFW score smaller than $0.2$ indicates the images are highly likely to be “safe-for-work”. JourneyDB gets an average NSFW score of $0.008$, where $99.01\%$ images get scores smaller than $0.2$ (safe for work), and only $0.16\%$ are greater than $0.8$. We manually go through these images, and find out and remove around $132$ images indeed unsuitable for work from the dataset.

We hope our efforts will contribute to the meticulous cleansing of the dataset, thereby providing a sanitized and non-violent dataset for the community.

\subsection*{Does the dataset relate to people?}
\noindent Yes, a subset of data is filtered by people.

\subsection*{Does the dataset identify any subpopulations (\eg by age, gender)?}

\noindent No.

\subsection*{Is it possible to identify individuals (\ie one or more natural persons), either directly or indirectly (\ie in combination with other data) from the dataset?}
\noindent No.

\subsection*{Does the dataset contain data that might be considered sensitive in any way (\eg data that reveals racial or ethnic origins, sexual orientations, religious beliefs, political opinions or union memberships, or locations; financial or health data; biometric or genetic data; forms of government identification, such as social security numbers; criminal history)?}

The dataset might contain a few sensitive data, because the prompts are collected from users. The distribution basically follows the Discord community.

\subsection*{What experiments were initially run on this dataset? Have a summary of those results.}
\noindent 
Based on our dataset, we set up four benchmarks, \ie prompt inversion, style retrieval, image caption, and visual question answering.

\subsection{\centering Data Collection Process}

\subsection*{How was the data associated with each instance acquired?}

\noindent
Each instance contains prompts and generated images, along with annotations of prompt classification (into content styles), image caption, and visual question answering.

\subsection*{What mechanisms or procedures were used to collect the data (\eg hardware apparatus or sensor, manual human curating, software program, software API)?}
\noindent We use software programs to collect the data.

\subsection*{If the dataset is a sample from a larger set, what was the sampling strategy (\eg deterministic, probabilistic with specific sampling probabilities)?}

\noindent  The dataset is not a sample of a larger set. 

\subsection*{Who was involved in the data collection process (\eg students, crowd-workers, contractors) and how were they compensated (\eg
how much were crowdworkers paid)?}

\noindent  We hire 40 professional annotators for prompt filtering. They earn roughly $\$50$ a day.

\subsection*{Over what time-frame was the data collected?}
\noindent %
The dataset was collected between 2023-02-01 and 2023-05-30.

\subsection*{Were any ethical review processes conducted (\eg by an institutional review board)?}
\noindent No official process is conducted.

\subsection*{Does the dataset relate to people?}
\noindent No.

\subsection{\centering Data Preprocessing}
\subsection*{What preprocessing/cleaning was done? (\eg discretization or bucketing, tokenization, part-of-speech tagging, SIFT feature extraction, removal of instances, processing of missing values)?}
\noindent We use the original image generated by Midjourney, and clean the prompts by removing specific words for Midjourney.

\subsection{\centering Uses}
\subsection*{Has the dataset been used for any tasks already? If so, please provide a description.}
\noindent As described in the paper, this dataset has been used to evaluate the performance of state-of-the-art visual-language models on generated contents.

\subsection*{Is there a repository that links to any or all papers or systems that use the dataset?}
\noindent
Yes, we will summarise some popular papers that use our dataset on our GitHub repository.

\subsection*{What (other) tasks could the dataset be used for?}
\noindent 
As introduce in section 4 in the main paper, the dataset could be used for many downstream tasks like prompt inversion, style retrieval, image caption and visual question answering.

\subsection*{Is there anything about the composition of the dataset or the way it was collected and preprocessed/cleaned/labeled that might impact future uses?}
\noindent Yes. There might be some misalignment between the prompts and the generated image, which may bring noise to the annotation.

\subsection*{Are there tasks for which the dataset should not be used?}
\noindent No

\subsection{\centering Data Distribution}
\subsection*{Will the dataset be distributed to third parties outside of the entity (\eg company, institution, organization) on behalf of which
the dataset was created? If so, please provide a description}
\noindent Yes. Anyone on the Internet can request for the data. %

\subsection*{How will the dataset be distributed? (\eg tarball on website, API, GitHub; does the data have a DOI and is it archived redundantly?)}
\noindent We plan to design the request mechanism. Users will submit a form and we will provide the downloading link. %

\subsection*{When will the dataset be distributed?}
\noindent Before 2023-06-30.

\subsection*{Will the dataset be distributed under a copyright or other intellectual property (IP) license, and/or under applicable terms of use (ToU)?}
\noindent We will provide a terms of use agreement with the dataset. The dataset as a whole will be distributed under a non-commercial license. %

\subsection*{Have any third parties imposed IP-based or other restrictions on
the data associated with the instances? If so, please describe these restrictions, and provide a link or other access point to, or otherwise reproduce, any relevant licensing terms, as well as any fees associated
with these restrictions.}
\noindent No.

\subsection*{Do any export controls or other regulatory restrictions apply to
the dataset or to individual instances? If so, please describe these
restrictions, and provide a link or other access point to, or otherwise
reproduce, any supporting documentation.}
\noindent No.

\subsection{\centering Dataset Maintenance}
\subsection*{Who is supporting/hosting/maintaining the dataset?}
\noindent The authors of this paper are maintainers of this dataset.

\subsection*{How can the owner/curator/manager of the dataset be contacted
(\eg email address)?}
\noindent By email.

\subsection*{Is there an erratum?}
\noindent At this time, we are not aware of errors in our dataset.

\subsection*{Will the dataset be updated? If so, how often and by whom? 
How will updates be communicated? (\eg mailing list, GitHub)}
\noindent We will check the GitHub issue after release. Users and also email us.
The dataset will be updated by the authors on an at-will basis (but no more than once a month).

\subsection*{If the dataset relates to people, are there applicable limits on the
retention of the data associated with the instances (\eg were individuals in question told that their data would be retained for a
fixed period of time and then deleted)? If so, please describe these
limits and explain how they will be enforced.}
\noindent No such limits are established.

\subsection*{Will older versions of the dataset continue to be supported/hosted/maintained?}
\noindent N/A

\subsection*{If others want to extend/augment/build on this dataset, is there a mechanism for them to do so? If so, is there a process for tracking/assessing the quality of those contributions. What is the process for communicating/distributing these contributions to users?}
\noindent It would be open for non-commercial usage.
